# Supplementary material for: Exploring Low-Resource Medical Image Classification with Weakly Supervised Prompt Learning
Source: arXiv:2402.03783 source file (2024-02-06)
Supplement: Supplementary file 1 [file Supplementary_material.pdf]

# Exploring Low-Resource Medical Image Classification with Weakly Supervised Prompt Learning —— Supplementary Material

## A. Comparison of zero-shot classification accuracy of different manual prompts and automatic prompts generated by our model on four datasets

Figure 1 compares the zero-shot classification accuracy of different manual prompts and automatic prompts generated by our model on four datasets. It can be seen that different manual prompts can lead to highly different zero-shot classification performances, which means that the quality of manual prompts has a direct and significant impact on model performance. This further indicates that the design of manual prompts depends heavily on domain experts. The method we proposed to automatically generate prompts can alleviate this dependency.

## B. Comparison of training and test loss curves, accuracy curves, ROC curves of our proposed models, and additional evaluations on the effect of the learnable components of our prompt generator

*(1) Loss curves and accuracy curves*

Taking 16-shot image classification as an example, we compared the training loss and test loss, as well as the training accuracy and test accuracy of

| Dataset | Class | Prompt | Accuracy |
|---|---|---|---|
| CheXpert 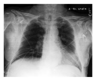 | Atelectasis | minimal retrocardiac atelectasis at the bilateral lung bases | 0.6000 |
| | Cardiomegaly | cardiac silhouette size is upper limits of normal | |
| | Consolidation | increased reticular consolidation at the right lower lobe | |
| | Edema | mild pulmonary edema | |
| | Pleural Effusion | small right bilateral pleural effusion | |
| | Atelectasis | trace atelectasis at the right lung base | 0.6030 |
| | Cardiomegaly | cardiomegaly which is unchanged | |
| | Consolidation | improved partial consolidation at the left upper lobe | |
| | Edema | improvement in pulmonary edema | |
| | Pleural Effusion | stable right bilateral pleural effusion | |
| | Atelectasis | mild trace atelectasis at the left lung zone | 0.6070 |
| | Cardiomegaly | redemonstration of cardiomegaly | |
| | Consolidation | partial consolidation at the left lower lobe | |
| | Edema | improvement in pulmonary edema | |
| | Pleural Effusion | decreased left subpulmonic pleural effusion | |
| | —— | $[V]_1 [V]_2 \ldots [V]_m$ [CLASS] | 0.6220 |

| Dataset | Class | Prompt | Accuracy |
|---|---|---|---|
| MIMIC-CXR 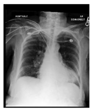 | Atelectasis | linear atelectasis at the left lung zone | 0.5390 |
| | Cardiomegaly | ap erect chest radiograph demonstrates the heart size is the upper limits of normal | |
| | Consolidation | improved bilateral consolidation at the left upper lobe | |
| | Edema | moderate pulmonary interstitial edema | |
| | Pleural Effusion | right bilateral pleural effusion | |
| | Atelectasis | minimal bandlike atelectasis at the upper lung zone | 0.5420 |
| | Cardiomegaly | heart size is borderline enlarged | |
| | Consolidation | retrocardiac consolidation at the right lower lobe | |
| | Edema | moderate pulmonary edema | |
| | Pleural Effusion | decreased right bilateral pleural effusion | |
| | Atelectasis | residual atelectasis at the bilateral lung bases | 0.5460 |
| | Cardiomegaly | cardiac silhouette size is mildly enlarged | |
| | Consolidation | increased reticular consolidation at the lower lung zone | |
| | Edema | moderate trace interstitial edema | |
| | Pleural Effusion | left bilateral pleural effusion | |
| | —— | $[V]_1 [V]_2 \ldots [V]_m$ [CLASS] | 0.5720 |

| Dataset | Class | Prompt | Accuracy |
|---|---|---|---|
| COVID 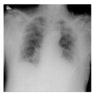 | Normal | cardiomediastinal silhouette is stable given differences in positioning | 0.5680 |
| | COVID | patchy ground glass consolidation in peripheral | |
| | Normal | in addition, there is thickening along the right pleura at the anterior junction line | 0.7540 |
| | COVID | confluent ground glass consolidation in lower | |
| | Normal | multilevel degenerative changes with marginal osteophyte formation of the thoracic spine are noted with mild dextroconvex curvature of the mid-to-lower thoracic spine | 0.7583 |
| | COVID | patchy ground glass consolidation in mid | |
| | —— | $[V]_1 [V]_2 \ldots [V]_m$ [CLASS] | 0.7997 |

| Dataset | Class | Prompt | Accuracy |
|---|---|---|---|
| RSNA 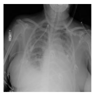 | Normal | the cardiomediastinal silhouette is stable | 0.4350 |
| | Pneumonia | mycoplasma at the left lower lobe | |
| | Normal | there are a probable trace left pleural effusion | 0.4859 |
| | Pneumonia | mycoplasma at the mid lung zone | |
| | Normal | compared with the prior studies, mild pulmonary vascular congestion is new | 0.7462 |
| | Pneumonia | viral at the lung bases | |
| | —— | $[V]_1 [V]_2 \ldots [V]_m$ [CLASS] | 0.7284 |

Figure 1: Comparison of zero-shot classification accuracy of different manual prompts and automatic prompts generated by our model on four datasets.

our final proposed model on the four datasets, as shown in Figure 2 and Figure 3. It can be observed from the figures that overall, both the training loss and the test loss show a downward trend, while the training accuracy and test accuracy show a gradual upward trend. Although the test loss is a bit higher than the training loss, combined with the fact that the test accuracy is overall similar to the training accuracy, it can be concluded that the model is well trained and well fitted. In addition, it can be observed that the

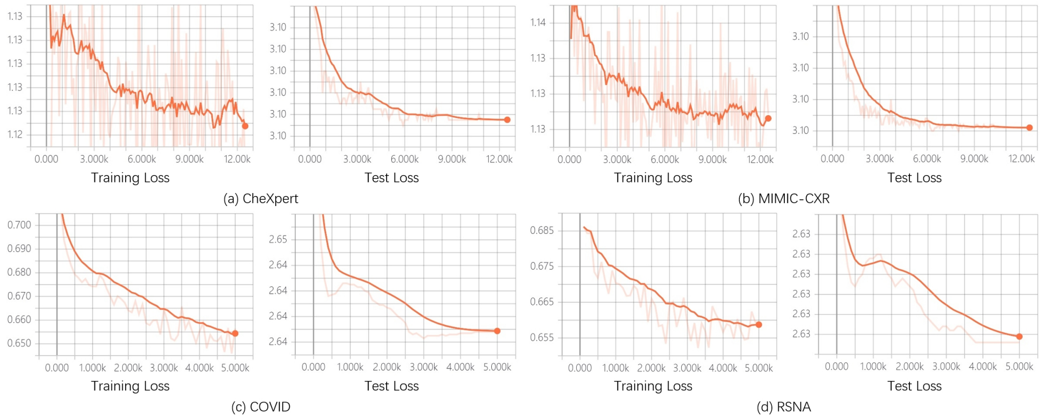


Figure 2: Comparison of training loss and test loss of our proposed model on four datasets, taking 16-shot image classification as an example.

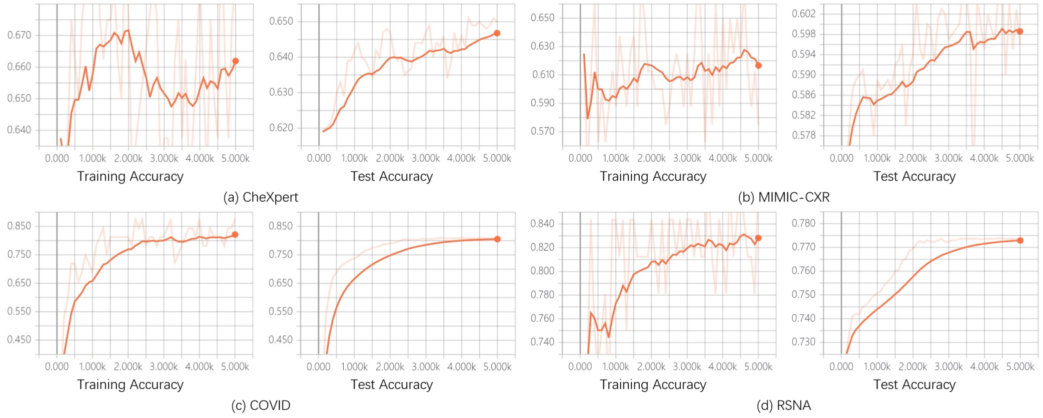


Figure 3: Comparison of training accuracy and test accuracy of our proposed model on four datasets, taking 16-shot image classification as an example.

training accuracy curve oscillates strongly on CheXpert and MIMIC-CXR, which is due to the fact that we only used 16 random samples for few-shot learning during training, so the training accuracy is greatly affected by these 16 samples.

Also, taking 16-shot image classification as an example, we compared the

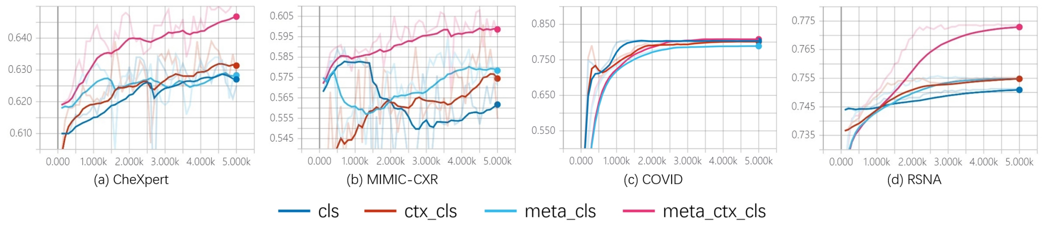


Figure 4: Comparison of test accuracy of models using our prompt generator with different learnable components on four datasets, taking 16-shot image classification as an example. 'cls', 'ctx_cls', 'meta_cls', and 'meta_ctx_cls' represent model with only class embeddings, model with context embeddings and class embeddings, model with Meta-Net and class embeddings, and model with all the learnable components, which is our proposed prompt generator, respectively.

test accuracy of models using our prompt generator with different learnable components, as shown in Figure 4. It can be observed that overall, the model with all learnable components (our proposed model) exhibits the best accuracy, while the accuracy of the model with only class embeddings is the least ideal, which is consistent with the performance comparison and analysis conclusions of these four models in Subsection 4.5.2.

*(2) ROC curves*

Taking 16-shot image classification as an example, we compared the training ROC curves and test ROC curves of our final proposed model and the test ROC curves of the models using our prompt generator with different learnable components, as shown in Figure 5. Since there are too many ROC curves for the multi-classification task, here we only take COVID and RSNA as examples, omitting the ROC curves for the other two multi-category datasets. It can be observed that the area under the curve is large for both the training ROC and test ROC, and the test ROC tends to be closer to the train-

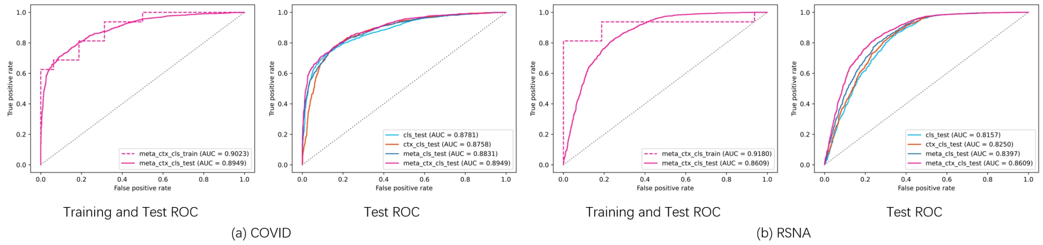


Figure 5: Training ROC and test ROC curves of our proposed model, and test ROC curves of the models using our prompt generator with different learnable components, taking 16-shot image classification as an example. 'cls', 'ctx_cls', 'meta_cls', and 'meta_ctx_cls' represent model with only class embeddings, model with context embeddings and class embeddings, model with Meta-Net and class embeddings, and model with all the learnable components, which is our proposed prompt generator, respectively.

ing ROC, indicating that the model is well-trained and well-fitted, with a high true-positive rate and low false-positive rate. Furthermore, it can be observed that overall, the model with all learnable components (our proposed model) exhibits the best area under the curve, whereas the model with context embeddings component and the model with meta embeddings component both exhibit better area under the curve than the model with only class embeddings. This is consistent with the performance comparison and analysis conclusions of these four models in Subsection 4.5.2.

*(3) More evaluation metrics*

Taking 16-shot image classification as an example, we compared the performance of the models using our prompt generator with different learnable components, measured by precision, specificity, sensitivity, and F1-Score. Here we report the macro average values of these metrics, as shown in Table 1. It can be observed that overall, the performance of the model with all

learnable components added (our proposed model) is the best, while adding context embeddings and Meta-Net components individually also brings significant performance improvements, which is consistent with the experimental results in Subsection 4.5.2.

| Dataset | Model | Precision | Specificity | Sensitivity | F1-Score |
|---|---|---|---|---|---|
| CheXpert | cls | 0.6313 | 0.6320 | 0.6140 | 0.9003 |
| | ctx_cls | 0.6567 | 0.6470 | 0.6422 | 0.9125 |
| | meta_cls | 0.6424 | 0.6400 | 0.6267 | 0.9053 |
| | meta_ctx_cls | **0.6589** | **0.6580** | **0.6566** | **0.9145** |
| MIMIC-CXR | cls | 0.6147 | 0.6010 | 0.5846 | 0.8918 |
| | ctx_cls | 0.6219 | 0.5950 | 0.5862 | 0.8955 |
| | meta_cls | 0.6259 | 0.5930 | 0.5922 | 0.8985 |
| | meta_ctx_cls | **0.6337** | **0.6110** | **0.6099** | **0.9028** |
| COVID | cls | 0.8068 | 0.8026 | 0.8027 | 0.8026 |
| | ctx_cls | 0.8045 | 0.8040 | 0.8041 | 0.8040 |
| | meta_cls | 0.8108 | 0.8074 | 0.8076 | 0.8074 |
| | meta_ctx_cls | **0.8117** | **0.8080** | **0.8082** | **0.8080** |
| RSNA | cls | 0.7548 | 0.7516 | 0.7508 | 0.7516 |
| | ctx_cls | 0.7822 | 0.7753 | 0.7524 | 0.7340 |
| | meta_cls | 0.7869 | 0.7623 | 0.7520 | 0.7524 |
| | meta_ctx_cls | **0.7909** | **0.7784** | **0.7760** | **0.7784** |

Table 1: Performance of the models using our prompt generator with different learnable components, measured by precision, specificity, sensitivity, and F1-Score, taking 16-shot image classification as an example. 'cls', 'ctx_cls', 'meta_cls', and 'meta_ctx_cls' represent model with only class embeddings, model with context embeddings and class embeddings, model with Meta-Net and class embeddings, and model with all the learnable components, which is our proposed prompt generator, respectively. We only report the macro average of the metrics. The best results are in bold.

In addition, we also visualized the confusion matrixes of our proposed model on the four datasets, as shown in Figure 6.

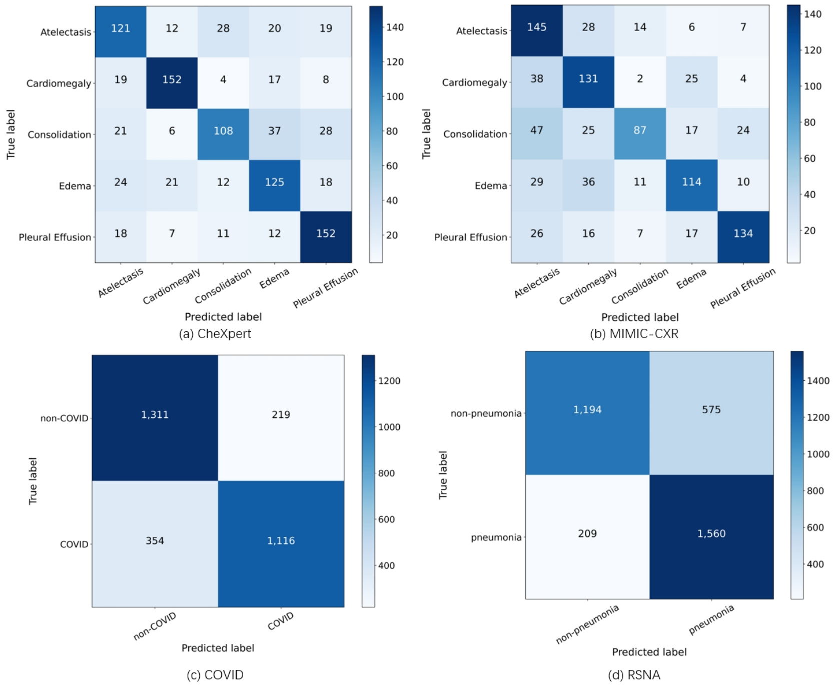


Figure 6: Confusion matrixes of our proposed model on four datasets, taking 16-shot image classification as an example.
